# Supplementary material for: Survey on Disaster Management Datasets for Remote Sensing Based Emergency Applications
Source: arXiv:2605.08196 source file (2026-05-05)
Supplement: Supplementary file 1 [file appendices.tex]

%---------------definitions---------
% \subsection{Definitions}
\begin{itemize}
\item \textbf{Disaster}: A disaster is a significant and devastating disruption to the functioning of a community where the capacity of that community is insufficient to cope or recover with its own resources. % Disasters can be caused naturally, man-made, and technological hazards, as well as various factors that influence the exposure and vulnerability of a community.\cite{www.ifrc.org}
\vspace{.2cm}

\item \textbf{Natural Disaster}:  A disaster caused by natural factors called as a natural disaster e.g., earthquake, flood, cyclone \cite{alexander2018natural}.
\vspace{.2cm}

\item \textbf{Man-made disaster}:  A disaster caused because of human activities. Examples may include wars, fire accidents, industrial accidents \cite{mohamed2007overview}.
\vspace{.2cm}
 
\item \textbf{Disaster Management}: is a process of effectively preparing for and responding to disasters. It involves strategically organizing resources to lessen the harm that disasters cause. It also involves a systematic approach to managing the responsibilities of \textbf{disaster prevention}, \textbf{preparedness}, \textbf{response}, and \textbf{recovery} as part of disaster management cycle \cite{alexander2015disaster}.
\vspace{.2cm}  

\item \textbf{Disaster response}:  refers to the actions taken directly before, during or in the immediate aftermath of a disaster \cite{alexander2015disaster}. It can include evacuations, search and rescue missions, and emergency medical assistance. The objective is to save lives, ensure health and safety and to meet the subsistence needs of the people affected.
\vspace{.2cm}

\item \textbf{Geographic Information Systems (GIS):} are computer based tools to manage, analyze, edit, output, and visualize geographic data\cite{burrough2015principles}. GIS store, analyze, and visualize data for geographic positions on Earth’s surface. GIS stands for Geographic Information Systems and is a computer-based tool that examines spatial relationships, patterns, and trends in geography.
\vspace{.2cm}

\item \textbf{Remote Sensing}: the process of detecting and monitoring the physical characteristics of an area by measuring its reflected and emitted radiation at a distance (typically from satellite or aircraft) \cite{zhu2018review}.The collected data is then processed and analyzed to generate valuable information about various aspects of the environment.
\vspace{.2cm}

\item \textbf{NAIP}: National Agricultural Imagery Program, acquires aerial imagery during the agricultural growing seasons in the continental United States\cite{davies2010estimating}. It is administered by the USDA's Farm Service Agency through the Aerial Photography Field Office in Salt Lake City.
\vspace{.2cm}

\item \textbf{Geodata}: Geodata is location information stored in a GIS\cite{teixeira2018qualitative}. By viewing data with a geographic component, we see it through a different lens.
\vspace{.2cm} 

\item \textbf{GIS Mapping}: It was used back in 1854 to map a disease outbreak in the City of London. Fundamentally, we still use this type of spatial analysis today but in a more sophisticated way. In a nutshell, data without spatial reference doesn’t provide geographic context\cite{burrough2015principles}. And without geographic context, you can’t fully understand the world that we live in today.
\vspace{.2cm}

\item \textbf{SpatioTemporal Asset Catalog (STAC)}:
The Spatio-temporal Asset Catalog (STAC) specification provides a common structure for describing and cataloging spatiotemporal assets\cite{9553518}. A spatio-temporal asset is any file that represents information about the earth captured in a certain space and time.
\vspace{.2cm}

\item \textbf{UNISDR}: United Nations Office for Disaster Risk Reduction
\vspace{.2cm} 

\item \textbf{NDVI}: Normalized difference vegetation index is used in understanding vegetation density and assessing changes in plant health. NDVI is calculated as a ratio between the red (R) and near infrared (NIR) values in traditional fashion: (NIR - R) / (NIR + R)
\vspace{.2cm}

\end{itemize}
